# Supplementary material for: Seminaive Materialisation in DatalogMTL
Source: arXiv:2208.07100 source file (2022-09-27)
Supplement: Supplementary file 1 [file appendix.tex]

\section{Technical Appendix}

\subsection{Proofs for \Cref{subsec:seminaive}}

To prove the results from this section, it is  convenient to make the following additional observation about the relation between $\mathcal{N}$ and $\Delta$ in our procedure:

% \noindent\textbf{\Cref{lemma_delta}:} 
\begin{proposition}\label{lemma_delta}
At the start of each iteration of the loop in Procedure~\ref{alg::seminaive}, 
it holds that $(\D' \doublecup \mathcal{N}) = ( \D' \doublecup \Delta)$.
\end{proposition}
\begin{proof}
Initially, $\mathcal{N} = \emptyset$ and $\Delta = \D' =\D$, so the statement of the proposition holds at the start of
the first iteration. We next consider further iterations.

To show that $(\D' \doublecup \mathcal{N}) \subseteq ( \D' \doublecup \Delta )$, we assume that $\D' \doublecup \mathcal{N} \models M@t$, for some relational fact $M@t$. Therefore, we have either $\D' \models M@t$, or $\D' \not\models M@t$ and ${\mathcal{N} \models M@t}$.
If $\D' \models M@t$, then clearly $\D' \doublecup \Delta \models M@t$.
Next, consider the case when
${\D' \not\models M@t}$ and
$\mathcal{N} \models M@t$. 
Since $\mathcal{N} \models M@t$, we have also  $\D' \doublecup \mathcal{N} \models M@ t$.
Thus,
there need to exist intervals $\varrho'$ and $\varrho''$, both of which include $t$, and such that $M@\varrho' \in \mathcal{N}$,  $M@\varrho'' \in \D' \doublecup \mathcal{N}$, and $\varrho' \subseteq \varrho''$.
Hence,
$M@\varrho'' \models M@\varrho'$, and so, 
by the definition of $\Delta$ in Line~\ref{alg2_delta}, we obtain that $M@\varrho'' \in \Delta$.
Therefore $\Delta \models M@t$, and thus, $\D' \doublecup \Delta \models M@t$.

To show that $(\D' \doublecup \Delta ) \subseteq ( \D' \doublecup \mathcal{N}) $, we assume that $\D' \doublecup \Delta \models M@t$, for some relational fact $M@t$. Therefore, we have $\D' \models M@t$ or $\Delta \models M@t$.
If $\D' \models M@t$, then  $\D' \doublecup \mathcal{N} \models M@t$.
Otherwise, $\Delta \models M@t$, and so, 
there needs to exist $\varrho$ such that $t \in \varrho$ and $M@\varrho \in \Delta$. 
By the definition of $\Delta$ in Line~\ref{alg2_delta}, we have $\Delta \subseteq \D' \doublecup \mathcal{N}$, so $M@\varrho \in (\D' \doublecup \mathcal{N})$, and therefore $\D' \doublecup \mathcal{N} \models M@t$.
\end{proof}

\bigskip
\noindent\textbf{\Cref{soundness_sm}}~\textbf{(Soundness):}  Consider Procedure \ref{alg::seminaive} running on input  $\Prog$ and $\D$. 
Upon the completion of the $k$th (for some $k 
\in \N$) iteration of the loop of  Procedure~\ref{alg::seminaive}, 
it holds that  $\I_{\D'} \subseteq  T_{\Prog}^{k}(\I_\D)$.

\begin{proof}
For each $k \in \N$, we let  $\mathcal{N}_k$,  $\Delta_k$, and $\D_k$ denote the contents of, respectively,  $\mathcal{N}$,  $\Delta$, and $\D'$ in Procedure~\ref{alg::seminaive} upon the completion of the $k$th iteration of the loop.
Thus, it suffices to show,  inductively on  $k \in \N$, that $\I_{\D_k} \subseteq T_\Prog^k(\I_\D)$. 

In the base case, by the initialisation of the procedure,  we have $\D_0 = \D$.
Moreover, ${T_\Prog^0(\I_\D) = \I_{\D} }$, and so, $\I_{\D_0} \subseteq T_\Prog^0(\I_\D)$, as required.

For the inductive step, we assume that $\I_{\D_k} \subseteq  T_{\Prog}^{k}(\I_\D)$, for some $k \in \N$, and that the procedure enters the $k+1$st iteration of the loop.
If  the $k+1$st iteration of the loop breaks in Line~\ref{alg2_7}, then $\D_{k+1}=\D_{k}$.
By the inductive assumption we have
${ \I_{\D_{k}} \subseteq  T_{\Prog}^{k}(\I_\D) }$,
so ${ \I_{\D_{k+1}} \subseteq  T_{\Prog}^{k}(\I_\D) }$, and thus,
 ${ \I_{\D_{k+1}} \subseteq  T_{\Prog}^{k+1}(\I_\D) }$.

Now, assume that the $k+1$ iteration of the loop does not break in Line~\ref{alg2_7}.
To show that
${ \I_{\D_{k+1}} \subseteq  T_{\Prog}^{k+1}(\I_\D) }$, we assume that 
$\I_{\D_k+1} \models  M@t$, for some relational fact $M@t$.
By Line~\ref{alg2_delta}, we obtain that $\D_{k+1} = \D_{k} \doublecup \mathcal{N}_{k+1}$.
Therefore, we have
$\D_{k} \models M@t$
or 
$\mathcal{N}_{k+1} \models M@t$.
\begin{itemize}
    \item[Case 1:] \emph{$\D_k \models M@t$}. 
    By the inductive assumption, we know that
    $\I_{\D_k}\subseteq T_{\Prog}^{k}(\I_\D)$,
     so $T_{\Prog}^{k}(\I_\D) \models  M@t$.
    Clearly,  $T_{\Prog}^{k}(\I_\D) \subseteq T_{\Prog}^{k+1}(\I_\D) $,  so 
     $T_{\Prog}^{k+1}(\I_\D) \models  M@t$.
    
    \item[Case 2:] \emph{$\mathcal{N}_{k+1} \models M@t$}. 
    By Line~\ref{alg2_5}, we have $\mathcal{N}_{k+1} = \semi{\Prog}{\D_k}{\Delta_k}$.
    Thus, by \Cref{def::semi-inst}, there is a rule $r \in \Prog$, say of  the form ${ M' \gets M_1 \land \dots \land M_n }$, such that $\ins{r}{\D_k \threedotcolon \Delta_k } \models M@t$.
    Hence, by Expression~\eqref{eq:rel-instance-delta}, there are  a substitution $\sigma$ and  
    intervals $\varrho_1, \dots, \varrho_n$ such that $(\matA_1\sigma@\varrho_1 , \dots , \matA_n \sigma@\varrho_n) \in \ins{r}{\D_k\threedotcolon \Delta_k}$ and
    ${M'\sigma@(\varrho_1 \cap \dots \cap \varrho_n) \models M@t}$.
    Since $(M_1\sigma@\varrho_1 , \dots , M_n \sigma@\varrho_n)$ belongs to $\ins{r}{\D_k \threedotcolon \Delta_k}$,
    the sequence 
    $(M_1\sigma@\varrho_1 , \dots , M_n \sigma@\varrho_n)$ belongs also to $\ins{r}{\D_k}$.
    Therefore, by Expression~\eqref{eq:consequences},
    we obtain that $\D_k \models M_i @ \varrho_i$, for each  $i \in \{1, \dots, n \}$.
    Hence, by definition, $T_\Prog (\I_{\D_k}) \models M'\sigma@(\varrho_1 \cap \dots \cap \varrho_n) $, and so, $T_\Prog (\I_{\D_k}) \models M@t$.
    By the inductive assumption, we have  ${\I_{\D_k} \subseteq T_\Prog^k(\I_{\D})}$, therefore
    $T_{\Prog}^{k+1}(\I_\D) \models M@t$.  \qquad \qed
\end{itemize}
\end{proof}

\bigskip
\noindent\textbf{\Cref{complete_sm}}~\textbf{(Completeness):}  Consider Procedure \ref{alg::seminaive} running on input  $\Prog$ and $\D$. For each $k \in \N$, upon the completion of the $k$th iteration of the loop of  Procedure~\ref{alg::seminaive},
it holds that  $  T_{\Prog}^{k}(\I_\D) \subseteq \I_{\D'} $.

\begin{proof}
We  use the same notation $\mathcal{N}_k$, $\Delta_k$, and  $\D_k$ as in the proof of \Cref{soundness_sm}.
Let $\alpha$ be the least ordinal such that $T_{\Prog}^{\alpha}(\I_\D) = \can{\Prog}{\D}$, so ${T_{\Prog}^{\alpha}(\I_\D) = T_{\Prog}^{\alpha+1}(\I_\D)}$.
We will show, inductively on natural numbers $k \leq \alpha$, that $T_\Prog^k(\I_\D) \subseteq \I_{\D_k}$. The base case holds trivially, because  we have $\D_0 = \D$,  and so,  $T_\Prog^0(\I_\D) \subseteq \I_{\D_0} $.

For the inductive step, assume that  $T_{\Prog}^{k+1}(\I_\D) \models M@t$, for some relational fact $M@t$.
We show that $\I_{\D_{k+1}} \models  M@t$. 
If $T_{\Prog}^{k}(\I_\D) \models M@t$ then, by the inductive assumption, ${\I_{\D_k} \models M@t}$.
Since $\I_{\D_{k}} \subseteq \I_{\D_{k+1}}$, we obtain that  $\I_{\D_{k+1}} \models M@t$.
Now, assume that $T_{\Prog}^{k}(\I_\D) \not\models M@t$ and 
$T_{\Prog}^{k+1}(\I_\D) \models M@t$.
Hence,
there exists a rule $r\in \Prog$,
say of the form $M' \gets M_1 \land \dots \land M_n$, and a time point $t'$ such that an application of $r$ at $t'$ yields $M@t$.
More precisely, it means that there exists a
substitution $\sigma$
such that $T_{\Prog}^{k}(\I_\D) \models M_i \sigma @t'$, for each $i \in \{1, \dots, n \}$, and 
$M'\sigma @ t' \models M@t$. 
Next, for each $i \in \{1, \dots, n \}$, we let $\varrho_i$ be the subset-maximal interval such that $T_{\Prog}^{k}(\I_\D) \models M_i \sigma @ \varrho_i$ and $t' \in \varrho_i$. 
%(note that each $\varrho_i$ is non-empty). 
By the inductive assumption, we obtain that
$T_{\Prog}^{k}(\I_\D) \subseteq \I_{\D_k}$, so
${\D_k} \models M_i \sigma @ \varrho_i$, for each $i \in \{1, \dots, n \}$.
Hence, by Expression~\eqref{eq:consequences}, we have  $(M_1 \sigma @\varrho_1, \cdots, M_n \sigma @\varrho_n) \in \ins{r}{\D_k}$. 

We argue that
$(M_1 \sigma @\varrho_1, \cdots, M_n \sigma @\varrho_n) \in \ins{r}{\D_k \threedotcolon \Delta_{k} }$.
By Expression~\eqref{eq:rel-instance-delta}, it suffices to show that
there is $i \in \{1, \dots, n \}$ such that ${\D_k \setminus \Delta_k \not\models  M_i \sigma @ \varrho_i}$.
For this, we will consider two cases, namely, when $k=0$ and when $k >0$.
\begin{itemize}
\item[Case 1:] \emph{$k=0$}. 
Then, by the initialisation of Procedure~\ref{alg::seminaive}, we have  $\D_k \setminus \Delta_k = \emptyset$, so   $\D_k \setminus \Delta_k \not\models M_i \sigma @\varrho_i$, for each $i \in \{1, \dots, n \}$.

\item[Case 2:] \emph{$k > 0$}. 
By Line~\ref{alg2_8}, we have $\D_k = \D_{k-1} \doublecup \mathcal{N}_k$ so, by \Cref{lemma_delta}, we  obtain  $\D_k = \D_{k-1} \doublecup \Delta_k$.
Thus $\I_{\D_k} = \I_{\D_{k-1}} \cup \I_{\Delta_{k}}$, 
so ${ \I_{\D_k}\setminus \I_{\Delta_k} = \I_{\D_{k-1}} \setminus \I_{\Delta_k} }$, and therefore $\I_{\D_k}\setminus \I_{\Delta_k} \subseteq \I_{\D_{k-1}}$. 
Hence, it suffices to show that $\D_{k-1} \not\models M_i\sigma@\varrho_i$, for some $i \in \{1, \dots, n \} $.  
Suppose towards a contradiction that $\D_{k-1} \models M_i\sigma@\varrho_i$, for all $i \in \{1, \dots, n \}$. 
By  \Cref{soundness_sm},  $T_{\Prog}^{k-1}(\I_{\D}) \models M_i\sigma@\varrho_i$, for all $i \in \{1, \dots, n \}$.
Thus,
 $T_{\Prog}^{k}(\I_{\D}) \models M@t$, which raises a contradiction.
\end{itemize}
Finally, assume that $k > \alpha$.
By the inductive argument above and by \Cref{soundness_sm}, we obtain that $T_{\Prog}^{\alpha}(\I_{\D}) = \I_{\D_\alpha}$. 
Since $T_{\Prog}^{\alpha}(\I_\D) = \can{\Prog}{\D}$, we obtain that $\D_{\alpha+1} = \D_{\alpha}$. 
Thus, by Line~\ref{alg2_delta}, we obtain that $\Delta_{\alpha+1} = \emptyset$.
Consequently, 
Procedure \ref{alg::seminaive}  terminates in Line~\ref{alg2_7} in the $\alpha+1$st iteration of the loop, and  outputs $\D_{\alpha}$.
Since $T_{\Prog}^{\alpha}(\I_{\D}) = \I_{\D_\alpha}$, 
$T_{\Prog}^{\alpha}(\I_\D) = \can{\Prog}{\D}$, and $k > \alpha$, we  
obtain that $T_{\Prog}^{k}(\I_{\D}) = \I_{\D_\alpha}$.
Hence, $T_{\Prog}^{k}(\I_{\D}) \subseteq \I_{\D'}$, where $\D' = \D_\alpha$ is the output of the procedure. \qquad \qed
\end{proof}

\subsection{Proofs for \Cref{subsec:oseminaive}}

\noindent\textbf{\Cref{non-rec}:} Consider Procedure~\ref{alg::optseminaive} running on input $\Prog$ and $\D$ and let $\prognr$ be the non-recursive fragment of $\Prog$.
If $flag = 1$, then $\can{\prognr}{\D} \subseteq \I_{\D'}$.
\begin{proof}
If $\can{\prognr}{\D}$ entails a relational fact with a recursive predicate, then this fact is already entailed by $\I_\D$ and, by the form of 
Procedure~\ref{alg::optseminaive}, we have $\I_\D \subseteq \I_{\D'}$.
To show that the implication holds also for facts with non-recursive predicates, we observe that $\I_{\D} \subseteq \I_{\D'}$ and $\prognr \subseteq \Prog$ imply
$\can{\prognr}{\D}  \subseteq \can{\Prog}{\D'}$.
Hence, it suffices to show that each relational fact with non-recursive predicates which is satisfied in $\can{\Prog}{\D'}$
is also satisfied in
$\I_{\D'}$. 

According to Line~\ref{line:c} and Line~\ref{loopend} in Procedure 3, we know that $\D'$ will change to a bigger dataset~($\D' \doublecup \mathcal{N}$) after each iteration, where $\mathcal{N}$ is obtained in Line~\ref{line:n}. It suffices to show the case in which $\D'$ and $\mathcal{N}$ denotes the contents of  $\D'$ and $\mathcal{N}$ when $flag$ becomes 1 for the first time. Hence, we have $\D'$ and $\D'\doublecup \mathcal{N}$ entail same facts with non-recursive predicates in $\Prog$ according to Line~\ref{same}.
Before the flag changes to 1, Procedure~\ref{alg::optseminaive} works exactly as Procedure~\ref{alg::seminaive}, so we obtain that $\D'\doublecup \mathcal{N} = T_{\Prog}(\I_{\D'})$.
%
% According to Line~\ref{line:n} and \Cref{lemma_delta}, we obtain that $\D'\doublecup \mathcal{N} = T_{\Prog}(\I_{\D'})$\nb{How do we know that this equality is true? Line 3 does not tell it, it only tells us how $\mathcal{N}$ is defined. Some argument seems to be missing here.}.
%
Therefore, it suffices to show that both $T_{\Prog}(\I_{\D'})$ and $T_{\Prog}^2(\I_{\D'})$ entails the same 
facts with non-recursive predicates in $\Prog$, as applying the same argument recursively implies $\I_{\D'}$ and 
$\can{\Prog}{\D'}$ entail same facts with non-recursive predicates in $\Prog$. 
Towards a contradiction we suppose that $T_{\Prog}^2(\I_{\D'}) \models M@t$ for 
some relational fact $M@t$ with a non-recursive predicate in $\Prog$ and $T_{\Prog}(\I_{\D'}) \not\models M@t$. 
Hence, there is a rule $r \in \ground{\Prog}{\D}$ and a time point $t'$ such that $T_{\Prog}^1(\I_{\D'})$ entails 
each body atom of $r$ at $t'$, and the head of $r$ holding at $t'$ entails $M@t$. Since $M@t$ is a relational fact with a 
non-recursive predicate in $\Prog$ and according to Definition~\ref{def:nonrecursive}, we 
obtain that there is no path with a cycle ending in the non-recursive predicate node 
representing $M$, so we obtain that each body atom in $r$ should mentions only 
non-recursive predicates in $\Prog$. Recall that $\I_{\D'}$ and $T_{\Prog}^1(\I_{\D'})$ entails same facts with non-recursive 
predicates in $\Prog$, so $\I_{\D'}$ also entails each body atom of $r$ at $t'$, so $T_{\Prog}^1(\I_{\D'}) \models M@t$. Hence, $\I_{\D'} \models M@t$,  which raises a 
contradiction. 

\end{proof}

\noindent\textbf{\Cref{lemma:fb}:} If $\I_{\D}\mid_{(-\infty, t]} = T_{\Prog}(\I_{\D})\mid_{(-\infty, t]}$, for a forward propagating program $\Prog$, dataset $\D$, and  time point $t$,
then $\I_{\D}\mid_{(-\infty, t]} = \can{\Prog}{\D}\mid_{(-\infty, t]}$.
\begin{proof}
%We focus on a forward-propagating $\Prog$, as the backward-propagating case is analogous. 
It suffices to show that ${ T_{\Prog}(\I_{\D})\mid_{(-\infty, t]} = T_{\Prog}^{2}(\I_{\D})\mid_{(-\infty, t]} }$, as applying the same argument recursively implies
$\I_{\D}\mid_{(-\infty, t]} = \can{\Prog}{\D}\mid_{(-\infty, t]}$.
The inclusion $T_{\Prog}(\I_{\D})\mid_{(-\infty, t]} \subseteq T_{\Prog}^{2}(\I_{\D})\mid_{(-\infty, t]} $ is clear, so we proceed with the opposite direction.
Towards a contradiction we suppose  that $T_{\Prog}^{2}(\I_{\D}) \models M@t'$ and $T_{\Prog} (\I_{\D}) \not\models M@t'$,
for some relational fact $M@t'$ with
 $t' \in (-\infty, t]$.
Hence, there is a rule $r \in \ground{\Prog}{\D}$ and a time point $t''$ such that $T_{\Prog}(\I_{\D})$ satisfies each body atom of $r$ at  $t''$, and the head of $r$ holding at $t''$ entails $M@t'$.
Since $r$ is forward-propagating, we have $t''\leq t'$
so, by $t' \leq t$, we obtain that $t'' \leq t$.
Moreover, by the fact that $r$ mentions only past operators in its body, we obtain that  already 
$T_{\Prog} (\I_{\D})\mid_{(-\infty, t]} $ satisfies each body atom of $r$ at $t''$.
However, by the  assumption, 
$\I_{\D}\mid_{(-\infty, t]} = T_{\Prog}(\I_{\D})\mid_{(-\infty, t]}$,
so
$ \I_{\D}\mid_{(-\infty, t]} $ satisfies each body atom of $r$ at $t''$, and so, 
$T_{\Prog}(\I_{\D}) \models M@t'$, which raises a contradiction.
\end{proof}
\noindent\textbf{\Cref{lemma:invalid}:} If in  Procedure \ref{alg::optseminaive} a rule $r$ is removed from $\Prog'$ in Line 10 or in Line~15, then 
$\can{\Prog'}{\D' \doublecup \mathcal{N}} = \can{\Prog'\setminus 
\{r\}}{\D'\doublecup \mathcal{N}}$.
% \nb{P: please update tje statement of the lemma. DM: Adding the statement about the Line 10}
\begin{proof}
Clearly, $\can{\Prog'}{\D'\doublecup \mathcal{N}} \supseteq \can{\Prog'\setminus\{r\}}{\D'\doublecup \mathcal{N}}$, therefore
it is sufficient to show that ${\can{\Prog'}{\D'\doublecup \mathcal{N}} \subseteq \can{\Prog'\setminus\{r\}}{\D' \doublecup \mathcal{N}} }$. Suppose towards a contradiction that $\can{\Prog'}{\D' \doublecup \mathcal{N}} \not\subseteq \can{\Prog'\setminus\{r\}}{\D' \doublecup \mathcal{N}}$,
so
there is the least ordinal $\alpha$
such that 
${ T_{\Prog'}^{\alpha+1} (\I_{\D'\doublecup \mathcal{N}}) \models M@t }$ and ${ T_{\Prog' \setminus\{r \}}^{\alpha+1} (\I_{\D'\doublecup \mathcal{N}}) \not\models M@t }$, for some relational fact $M@t$.
So, 
there is a substitution $\sigma$ and a time point $t'$
such that---for 
$r$  of the generic form 
${ M' \gets M_1 \land \dots \land M_n }$---we have ${T_{\Prog'}^{\alpha}(\I_{\D' \doublecup \mathcal{N}}) \models M_i \sigma @ t'}$, for all $i \in \{ 1, \dots, n \}$, 
and $M'@t' \models M@t$.

If in Line~\ref{empty}, the condition in the \textbf{if} statement applies, then $r$ has  a
body atom $M_i$ that is non-recursive in $\Prog$ and such that $\D' \not\models M_i \sigma @ t'$.
Since 
$ \can{\Prog_{nr}}{\D} \subseteq \I_{\D'}$,
we get
$\can{\prognr}{\D} \not\models M_i \sigma @ t'$, and so, $\can{\Prog}{\D} \not\models M_i \sigma @ t'$.
Moreover, as $\Prog' \subseteq \Prog$ and ${\D' \doublecup \mathcal{N} = T_{\Prog'}(\I_{\D'})}$, we obtain
$T_{\Prog'}^{\alpha} (\I_{\D'\doublecup \mathcal{N}}) \subseteq
\can{\Prog}{\D}$. 
Thus $T_{\Prog'}^{\alpha} (\I_{\D' \doublecup \mathcal{N}}) \not\models M_i \sigma @ t'$,
which raises a contradiction.

Now, if in Line~\ref{proj}, the condition in the \textbf{if} statement applies, then $\Prog'$ is forward-propagating. By the construction of $t_r$ and the fact that  $r \in \Prog'$ is forward-propagating, we obtain that $t' \leq t_r$.
As all $M_i \sigma @ t'$ hold in $T_{\Prog'}^{\alpha}(\I_{\D' \doublecup \mathcal{N}})$, all these facts hold also in $\I_{\D'}$.
Therefore, 
$\I_{\D' \doublecup \mathcal{N}} \models M@t$ so $T_{\Prog' \setminus\{r \}}^{\alpha+1} (\I_{\D'\doublecup \mathcal{N}}) \models M@t$, which raises a contradiction.
\end{proof}

\noindent\textbf{\Cref{seminaive_theorem}}~\textbf{(Soundness and Completeness):} Consider Procedure \ref{alg::optseminaive} running on input  $\Prog$ and $\D$. For each $k \in \N$, the partial materialisation $\D'$ obtained upon completion of the $k$th iteration of the main loop represents the interpretation $T_{\Prog}^{k}(\I_{\D})$.
% \nb{P: please update the statement of the lemma.}

\begin{proof}
If for both Line~\ref{empty} and Line~\ref{proj}, the condition in the \text{IF} statement does not apply, then
Procedure~\ref{alg::optseminaive} works in the same way as Procedure~\ref{alg::seminaive} so, by \Cref{soundness_sm,complete_sm}, $\D'$ represents   $T_{\Prog}^{k}(\I_{\D})$.
If  $flag$ is changed to  $1$ in the $k$th iteration, then $\can{\prognr}{\D} \subseteq \I_{\D'}$, by \Cref{non-rec}.
Therefore,
${\can{\prognr}{\D} = \can{\Prog\setminus \prognr}{\D'}}$, and so,
$\prognr$ can be safely deleted from $\Prog$ in Line~\ref{delprognr}.

Otherwise, the loop from 
Procedure~\ref{alg::optseminaive} works similarly  as Procedure~\ref{alg::seminaive}, except that it deletes in Line~\ref{empty} or Line~\ref{proj} rules.
As we have shown in \Cref{lemma:invalid}, such rules 
can be safely deleted from the program, without loosing the properties established in \Cref{soundness_sm,complete_sm}.
\end{proof}
